# Supplementary material for: Let the Heads Talk: Beyond Diagonal Graph Attention
Source: arXiv:2610.01494 source file (2026-10-01)
Supplement: Supplementary file 1 [file A_Appendix.tex]

\newpage
\appendix
\input{preamble_appendix}

% From here on the table of contents collects entries again, so that the
% supplementary contents list shows the appendix only (see main.tex).
\etocsettocdepth.toc{subsubsection}

\begin{center}
    {\LARGE \bfseries TOPological Attention: Learning Cross-Head Communication on Graphs \par}
    \vspace{0.4em}
    {\Large Supplementary Material\par}
\end{center}

\vspace{1em}

\addcontentsline{toc}{part}{Supplementary Material}
\etocsetnexttocdepth{3}
\vspace{-1cm}
\localtableofcontents

\vspace{1em}
\input{chapters/appendix_a_additional_theory}
\input{chapters/appendix_b_proofs}
\input{chapters/appendix_c}
\input{chapters/appendix_d}
