# Supplementary material for: Let the Heads Talk: Beyond Diagonal Graph Attention
Source: arXiv:2610.01494 source file (2026-10-01)
Supplement: Supplementary file 2 [file appendix_a_additional_theory.tex]

\section{Additional Theory for the Transport Formalism}
\label{app:transport-formalism}

This appendix provides additional details for the directed transport
formalism introduced in Section~\ref{sec:background}. We clarify the
relationship between graph quivers, copresheaves, and path composition;
explain how directional transport is represented in the cellular-sheaf
realization; and relate the directed cross-incidence operator used in the
main text to the usual degree-zero sheaf Laplacian.


\subsection{Quiver representations and path composition}
\label{app:quiver-path-category}

Let
\[
    G=(\mathcal{V},\mathcal{E},s,t)
\]
be a directed graph, viewed as a quiver: each vertex \(i\in\mathcal{V}\) is
an object and each directed edge \(e\in\mathcal{E}\) is an arrow
\[
    e:s(e)\longrightarrow t(e).
\]
A representation of this quiver in
\(\mathbf{Vect}_{\mathbb{R}}\) assigns a vector space
\(\mathcal{Q}(i)\) to every vertex and a linear map
\[
    T_e:
    \mathcal{Q}(s(e))
    \longrightarrow
    \mathcal{Q}(t(e))
\]
to every directed edge. Following
\citet{hajij2025copresheaf}, we refer to this vector-space-valued
representation as a graph copresheaf.

The quiver has an associated \emph{path category}
\(\operatorname{Path}(G)\). Its objects are the vertices of \(G\), while its
morphisms are directed paths. If
\[
    p
    =
    (e_1,\ldots,e_k)
\]
is a path with
\[
    t(e_r)=s(e_{r+1})
    \qquad
    \text{for }r=1,\ldots,k-1,
\]
then the corresponding linear map is
\begin{equation}
    T_p
    =
    T_{e_k}\circ\cdots\circ T_{e_1}.
    \label{eq:appendix-path-composition}
\end{equation}
The empty path at a vertex \(i\) is the identity morphism
\(\operatorname{id}_i\), and the representation assigns to it
\begin{equation}
    T_{\operatorname{id}_i}
    =
    I_{\mathcal{Q}(i)}.
    \label{eq:appendix-path-identity}
\end{equation}
Thus a quiver representation extends canonically to a functor
\[
    \operatorname{Path}(G)
    \longrightarrow
    \mathbf{Vect}_{\mathbb{R}}.
\]

Importantly, the existence of arrows in both directions does not make them
inverses. If
\[
    e:j\to i,
    \qquad
    \bar e:i\to j
\]
are both present, the path-category construction imposes no requirement that
\begin{equation}
    T_{\bar e}T_e
    =
    I_{\mathcal{Q}(j)}
    \qquad\text{or}\qquad
    T_eT_{\bar e}
    =
    I_{\mathcal{Q}(i)}.
    \label{eq:appendix-no-inverse-requirement}
\end{equation}
Such identities would require additional algebraic relations that are not
part of the graph quiver used here. Likewise, two distinct directed paths
with the same source and target remain distinct morphisms in the free path
category unless further relations are explicitly imposed.

The path-category language therefore formalizes composition of local
transports without introducing reciprocity or invertibility assumptions.
For the message-passing layers studied in this work, the primitive
computational objects remain the single-edge maps \(T_e\); the path-category
extension describes how these maps compose mathematically. A single layer
does not explicitly evaluate all path maps, and in a deep neural network
successive edge transports are generally interleaved with nonlinearities and
state updates.


\subsection{State-dependent graph copresheaves}
\label{app:dynamic-copresheaf}

The edge maps in a neural network are generally not fixed throughout the
computation. At layer \(\ell\), the current network state
\(X^{(\ell)}\) may determine
\begin{equation}
    T_e^{(\ell)}
    =
    T_e^{(\ell)}
    \!\left(
        X^{(\ell)}
    \right).
    \label{eq:appendix-dynamic-edge-map}
\end{equation}
For any fixed \(X^{(\ell)}\), the collection
\[
    \left\{
        \mathcal{Q}^{(\ell)}(i),
        T_e^{(\ell)}(X^{(\ell)})
    \right\}_{i,e}
\]
defines an ordinary graph copresheaf. The term
\emph{dynamic graph copresheaf} used in the main text refers to the fact
that a new collection of edge maps is instantiated as the network state
changes.

Attention is an important example because its dependence is not purely
edge-local. For
\[
    e=(j\to i),
\]
the normalized coefficient
\[
    \alpha_{i\leftarrow j}^{(h)}
    =
    \frac{
        \exp s_{i\leftarrow j}^{(h)}
    }{
        \sum_{k\in\mathcal{N}(i)}
        \exp s_{i\leftarrow k}^{(h)}
    }
\]
depends on the other incoming scores at the same receiver. Consequently,
the instantiated edge map \(D_{i\leftarrow j}\) depends on the current
receiver neighborhood through the softmax normalization, even though it is
subsequently applied to the message carried by the individual edge
\(j\to i\).

This state dependence does not alter the algebraic statements in the main
text. They are statements about the collection of edge maps instantiated at
a fixed layer and forward pass.


\subsection{Directed edge cells and reciprocity}
\label{app:directed-sheaf-reciprocity}

Section~\ref{sec:background-sheaf} uses cellular sheaves to provide a
factorized realization of directed edge transport. We make the role of
directionality explicit here.

Consider first a single undirected edge
\[
    e=\{i,j\}
\]
with vertex stalks
\(\mathcal{F}(i)\), \(\mathcal{F}(j)\), edge stalk
\(\mathcal{F}(e)\), and restriction maps
\[
    F_{i\to e}:
    \mathcal{F}(i)\to\mathcal{F}(e),
    \qquad
    F_{j\to e}:
    \mathcal{F}(j)\to\mathcal{F}(e).
\]
Using the restriction-induced transport of
Section~\ref{sec:background-sheaf}, the source-to-target map from \(j\) to
\(i\) is
\begin{equation}
    T_{i\leftarrow j}
    =
    F_{i\to e}^{\top}
    F_{j\to e}.
    \label{eq:appendix-undirected-forward}
\end{equation}
Reversing the computational direction while using the same edge stalk and
the same pair of restriction maps gives
\begin{equation}
    T_{j\leftarrow i}
    =
    F_{j\to e}^{\top}
    F_{i\to e}
    =
    T_{i\leftarrow j}^{\top}.
    \label{eq:appendix-undirected-reverse}
\end{equation}
Thus a single undirected edge induces a reciprocity relation between the two
source-to-target operators.

This relation is not appropriate for a general attention layer, where
\(i\leftarrow j\) and \(j\leftarrow i\) are separate computational
interactions and their normalized attention operators need not be related.
We therefore represent the two computational directions, when both are
present, by distinct edge cells
\[
    e_{j\to i},
    \qquad
    e_{i\to j}.
\]
Each cell has its own restriction maps. For example,
\[
    S_{j\to i}:
    \mathcal{F}(j)\to\mathcal{F}(e_{j\to i}),
    \qquad
    R_{j\to i}:
    \mathcal{F}(i)\to\mathcal{F}(e_{j\to i})
\]
induces
\[
    T_{i\leftarrow j}
    =
    R_{j\to i}^{\top}S_{j\to i},
\]
whereas the reverse cell may independently use
\[
    S_{i\to j}:
    \mathcal{F}(i)\to\mathcal{F}(e_{i\to j}),
    \qquad
    R_{i\to j}:
    \mathcal{F}(j)\to\mathcal{F}(e_{i\to j})
\]
and hence
\[
    T_{j\leftarrow i}
    =
    R_{i\to j}^{\top}S_{i\to j}.
\]
No transpose relation between these two operators is then required.

The distinction is important: choosing an orientation for a single
undirected edge does not by itself create independent forward and reverse
transport. Independence arises because the two computational directions are
represented by distinct edge cells with independently instantiated
restriction maps.

Self-messages are not essential to this construction. When present in the
architectures considered here, they may be handled separately as nodewise
terms rather than through the directed edge-cell formalism.


\subsection{Global incidence operators}
\label{app:global-incidence}

The local factorizations
\[
    T_e
    =
    R_e^\top S_e
\]
can be assembled into global linear operators. Let
\[
    C^0(\mathcal{F})
    =
    \bigoplus_{i\in\mathcal{V}}
    \mathcal{F}(i),
    \qquad
    C^1(\mathcal{F})
    =
    \bigoplus_{e\in\mathcal{E}}
    \mathcal{F}(e)
\]
denote the direct sums of the vertex and edge stalks. Define
\[
    B_s,B_t:
    C^0(\mathcal{F})
    \longrightarrow
    C^1(\mathcal{F})
\]
by
\begin{equation}
    (B_sX)_e
    =
    S_eX_{s(e)},
    \qquad
    (B_tX)_e
    =
    R_eX_{t(e)}.
    \label{eq:appendix-incidence-definitions}
\end{equation}
With the standard Euclidean inner products on these direct sums, the
adjoint \(B_t^\ast\) gathers edge-space quantities at their target vertices.
Consequently,
\begin{align}
    \left(
        B_t^\ast B_sX
    \right)_i
    &=
    \sum_{e:t(e)=i}
    R_e^\top S_eX_{s(e)}
    \nonumber\\
    &=
    \sum_{e:t(e)=i}
    T_eX_{s(e)}.
    \label{eq:appendix-cross-incidence-action}
\end{align}
Thus
\begin{equation}
    \mathcal{A}_{\mathcal{F}}^{\rightarrow}
    :=
    B_t^\ast B_s
    \label{eq:appendix-directed-cross-incidence}
\end{equation}
is precisely the global source-to-target transport operator associated with
the directed edge maps \(T_e\).

Its adjoint is
\begin{equation}
    \left(
        \mathcal{A}_{\mathcal{F}}^{\rightarrow}
    \right)^\ast
    =
    B_s^\ast B_t,
    \label{eq:appendix-cross-incidence-adjoint}
\end{equation}
which transports along the complementary source--target incidence pattern.
In general,
\[
    B_t^\ast B_s
    \neq
    B_s^\ast B_t,
\]
so the directed transport operator need not be self-adjoint.


\subsection{Relation to the cellular-sheaf Laplacian}
\label{app:sheaf-laplacian-relation}

For an oriented one-dimensional cellular complex, the degree-zero cellular
coboundary can be written, under the conventions above, as
\begin{equation}
    \delta
    =
    B_t-B_s.
    \label{eq:appendix-coboundary}
\end{equation}
The corresponding degree-zero sheaf Laplacian is
\begin{align}
    L_{\mathcal{F}}
    &=
    \delta^\ast\delta
    \nonumber\\
    &=
    (B_t-B_s)^\ast(B_t-B_s)
    \nonumber\\
    &=
    B_t^\ast B_t
    +
    B_s^\ast B_s
    -
    B_t^\ast B_s
    -
    B_s^\ast B_t.
    \label{eq:appendix-sheaf-laplacian-expansion}
\end{align}
The two cross terms are therefore
\[
    B_t^\ast B_s
    \qquad\text{and}\qquad
    B_s^\ast B_t
    =
    (B_t^\ast B_s)^\ast.
\]

The architectures studied in this paper use the first of these terms
directly:
\[
    \mathcal{A}_{\mathcal{F}}^{\rightarrow}
    =
    B_t^\ast B_s.
\]
We do not construct the complete positive-semidefinite operator
\(L_{\mathcal{F}}\), nor do we evolve node features according to a sheaf
diffusion generated by \(L_{\mathcal{F}}\). The cellular-sheaf formalism is
used instead to expose an exact factorization of the local source-to-target
edge maps through restriction maps.

This distinction separates the role of the two formalisms used throughout
the paper. The graph-copresheaf map
\[
    T_e:
    \mathcal{Q}(s(e))
    \longrightarrow
    \mathcal{Q}(t(e))
\]
is the directed operator applied directly during message passing. Whenever
restriction maps \(S_e\) and \(R_e\) are specified, the cellular-sheaf
construction induces the same operator through
\[
    T_e
    =
    R_e^\top S_e.
\]
The attention and \textsc{TopA} constructions in
Sections~\ref{sec:attention-restriction-realization} and
\ref{sec:offdiag-sheaf-realization} give explicit instances of this
factorization.
