# Supplementary material for: Let the Heads Talk: Beyond Diagonal Graph Attention
Source: arXiv:2610.01494 source file (2026-10-01)
Supplement: Supplementary file 3 [file appendix_b_proofs.tex]

\section{Proofs and Structural Details}
\label{app:proofs-structural}

This appendix collects proofs and structural properties of the head-space
operators introduced in Sections~\ref{sec:representation} and
\ref{sec:native}. Unless stated otherwise, all statements concern the edge
operators instantiated at a fixed layer and network state.


\subsection{Proof of diagonal head-space transport}
\label{app:proof-attention-diagonal}

We first prove
Proposition~\ref{prop:attention-diagonal-transport}.

\begin{proof}[Proof of Proposition~\ref{prop:attention-diagonal-transport}]
For each directed edge \(e=(j\to i)\), the normalized multi-head attention
operator is
\[
    T_e^{\att}
    =
    D_e
    =
    \operatorname{Diag}
    \left(
        \alpha_e^{(1)},\ldots,\alpha_e^{(H)}
    \right).
\]
Acting on the stacked sender values
\(V_{s(e)}\in\R^{H\times C}\) gives
\[
    D_eV_{s(e)}
    =
    \begin{bmatrix}
        \alpha_e^{(1)}V_{s(e)}^{(1)}\\
        \vdots\\
        \alpha_e^{(H)}V_{s(e)}^{(H)}
    \end{bmatrix}.
\]
Summing over the incoming edges of receiver \(i\),
\begin{align}
    \sum_{e:t(e)=i}
    T_e^{\att}V_{s(e)}
    &=
    \sum_{e:t(e)=i}
    D_eV_{s(e)}
    \nonumber\\
    &=
    M_i^{\att},
\end{align}
which is precisely the pre-readout multi-head attention update in
Equation~\eqref{eq:mha}.

Since every \(D_e\) is diagonal, coordinate \(h\) of the sender value can
contribute only to coordinate \(h\) of the receiver representation:
\[
    \left[D_eV_j\right]^{(h)}
    =
    \alpha_e^{(h)}V_j^{(h)}.
\]
Thus normalized multi-head attention is a diagonal directed transport on the
head space realized by the architecture.
\end{proof}


\subsection{Proof of the restriction-induced realization of attention}
\label{app:proof-attention-sheaf}

We next prove
Proposition~\ref{prop:attention-restriction-realization}.

\begin{proof}[Proof of Proposition~\ref{prop:attention-restriction-realization}]
For normalized attention,
\[
    D_e
    =
    \operatorname{Diag}
    \left(
        \alpha_e^{(1)},\ldots,\alpha_e^{(H)}
    \right)
\]
has non-negative diagonal entries. Hence its principal square root
\[
    D_e^{1/2}
    =
    \operatorname{Diag}
    \left(
        \sqrt{\alpha_e^{(1)}},\ldots,
        \sqrt{\alpha_e^{(H)}}
    \right)
\]
is well defined and symmetric.

With
\[
    S_e
    =
    R_e
    =
    D_e^{1/2},
\]
the induced source-to-target transport is
\begin{align}
    R_e^\top S_e
    &=
    \left(D_e^{1/2}\right)^\top
    D_e^{1/2}
    \nonumber\\
    &=
    D_e^{1/2}D_e^{1/2}
    \nonumber\\
    &=
    D_e.
\end{align}
Consequently,
\begin{align}
    \left(
        B_t^\ast B_sV
    \right)_i
    &=
    \sum_{e:t(e)=i}
    R_e^\top S_eV_{s(e)}
    \nonumber\\
    &=
    \sum_{e:t(e)=i}
    D_eV_{s(e)}
    \nonumber\\
    &=
    M_i^{\att}.
\end{align}
Thus the restriction-induced cellular-sheaf transport reproduces the
attention update exactly.
\end{proof}

The square-root choice is only one possible factorization of \(D_e\). The
restriction maps above are introduced to realize the already instantiated
attention operator and are not additional parameters of the attention
mechanism.


\subsection{Native head basis and head relabeling}
\label{app:head-basis}

The diagonal characterization of attention is tied to the head decomposition
explicitly implemented by multi-head attention. It is therefore
basis-dependent in the ordinary linear-algebraic sense: an arbitrary change
of basis in \(\R^H\) need not preserve diagonality. What is intrinsic to the
architecture is the decomposition into \(H\) head coordinates.

The characterization is nevertheless closed under arbitrary relabelings of
those coordinates. Let \(P\in\R^{H\times H}\) be a permutation matrix and
define
\begin{equation}
    V_j'
    =
    PV_j,
    \qquad
    D_e'
    =
    PD_eP^\top.
    \label{eq:appendix-attention-head-permutation}
\end{equation}
Then
\begin{align}
    D_e'V_j'
    &=
    PD_eP^\top PV_j
    \nonumber\\
    &=
    PD_eV_j.
    \label{eq:appendix-attention-permutation-action}
\end{align}
Since conjugation by a permutation matrix only permutes the diagonal
entries, \(D_e'\) remains diagonal. Thus changing the labels assigned to the
heads changes only the coordinates used to describe the same headwise
transport structure.

At the network level, this statement should be understood as a simultaneous
relabeling of all head-indexed quantities and parameters. It does not claim
invariance to an arbitrary learned change of basis in head space.


\subsection{Structural properties of \textsc{TopA}}
\label{app:proof-offdiag-structural}

We now prove the two properties summarized in
Proposition~\ref{prop:offdiag-structural}.

\begin{proof}[Proof of Proposition~\ref{prop:offdiag-structural}]
Recall
\[
    T_e
    =
    D_e
    \left(
        I_H+\lambda\Omega_e
    \right)
    =
    D_e+\lambda D_e\Omega_e,
\]
where \(D_e\) is diagonal and
\(\operatorname{diag}(\Omega_e)=0\).

For any head \(h\),
\begin{align}
    (D_e\Omega_e)^{hh}
    &=
    \sum_{s=1}^{H}
    D_e^{hs}\Omega_e^{sh}
    \nonumber\\
    &=
    D_e^{hh}\Omega_e^{hh}
    \nonumber\\
    &=
    0,
\end{align}
because all off-diagonal entries of \(D_e\) vanish and
\(\Omega_e^{hh}=0\). Therefore
\[
    T_e^{hh}
    =
    D_e^{hh}
    =
    \alpha_e^{(h)}
\]
for every \(h\), proving
\[
    \operatorname{diag}(T_e)
    =
    \operatorname{diag}(D_e).
\]

If \(\Omega_e=0\), then immediately
\[
    T_e
    =
    D_e(I_H+\lambda 0)
    =
    D_e.
\]
Hence the complete aggregation becomes
\[
    M_i^{\offdiag}
    =
    \sum_{e:t(e)=i}
    D_eV_{s(e)}
    =
    M_i^{\att},
\]
which is exactly the vanilla attention update.
\end{proof}

Diagonal preservation is a statement about the operator instantiated at the
current layer and network state. Since \textsc{TopA} changes the hidden
representations passed to later layers, it may indirectly affect attention
coefficients computed at subsequent layers; the claim is only that the
routing residual does not alter the diagonal entries of the current
\(T_e\).


\subsection{Head relabeling for \textsc{TopA}}
\label{app:offdiag-head-permutation}

The \textsc{TopA} operator family inherits the permutation closure of the
underlying head decomposition.

Let \(P\in\R^{H\times H}\) be a permutation matrix and define
\begin{equation}
    D_e'
    =
    PD_eP^\top,
    \qquad
    \Omega_e'
    =
    P\Omega_eP^\top.
    \label{eq:appendix-offdiag-permutation-def}
\end{equation}
Conjugation by \(P\) permutes rows and columns simultaneously, so
\[
    \operatorname{diag}(\Omega_e')
    =
    0
\]
whenever
\(\operatorname{diag}(\Omega_e)=0\). The transformed edge operator is
\begin{align}
    T_e'
    &=
    D_e'
    \left(
        I_H+\lambda\Omega_e'
    \right)
    \nonumber\\
    &=
    PD_eP^\top
    \left(
        I_H+\lambda P\Omega_eP^\top
    \right)
    \nonumber\\
    &=
    PD_e
    \left(
        I_H+\lambda\Omega_e
    \right)
    P^\top
    \nonumber\\
    &=
    PT_eP^\top.
    \label{eq:appendix-offdiag-permutation}
\end{align}
For permuted sender values \(V_j'=PV_j\),
\begin{align}
    T_e'V_j'
    &=
    PT_eP^\top PV_j
    \nonumber\\
    &=
    PT_eV_j.
\end{align}
Thus the distinction between diagonal same-head transport and off-diagonal
cross-head transport is preserved under head relabeling.

This is a closure property of the operator family. It does not require the
particular generator \(g_\theta\) used in the implementation to be
permutation-equivariant: a corresponding relabeling of the model would also
require the head-indexed generator outputs and parameters to be relabeled
consistently.


\subsection{Magnitude of the residual transport}
\label{app:offdiag-residual-bound}

The bounded parameterization of \(\Omega_e\) gives a simple worst-case bound
on the magnitude of the additional transport. This result is not required
for the architecture, but makes explicit how the residual scale
\(\lambda\) controls the deviation from the diagonal operator.

From
\[
    \Omega_e
    =
    \operatorname{off}
    \left(
        \tanh g_\theta(\xi_e)
    \right),
\]
the elementwise \(\tanh\) implies
\begin{equation}
    |\Omega_e^{rs}|
    \leq
    1
    \qquad
    \text{for all }r,s,
    \label{eq:appendix-elementwise-bound}
\end{equation}
and
\(\Omega_e^{rr}=0\). Therefore at most \(H(H-1)\) entries can be
non-zero, giving
\begin{align}
    \|\Omega_e\|_F^2
    &=
    \sum_{\substack{r,s=1\\r\neq s}}^{H}
    |\Omega_e^{rs}|^2
    \nonumber\\
    &\leq
    H(H-1).
\end{align}
Hence
\begin{equation}
    \|\Omega_e\|_2
    \leq
    \|\Omega_e\|_F
    \leq
    \sqrt{H(H-1)}.
    \label{eq:appendix-omega-norm-bound}
\end{equation}

For normalized attention,
\[
    D_e
    =
    \operatorname{Diag}
    \left(
        \alpha_e^{(1)},\ldots,\alpha_e^{(H)}
    \right),
\]
with
\(0\leq\alpha_e^{(h)}\leq1\), and therefore
\begin{equation}
    \|D_e\|_2
    =
    \max_h\alpha_e^{(h)}
    \leq
    1.
    \label{eq:appendix-attention-norm-bound}
\end{equation}
Since
\[
    T_e-D_e
    =
    \lambda D_e\Omega_e,
\]
submultiplicativity of the operator norm gives
\begin{align}
    \|T_e-D_e\|_2
    &=
    \lambda
    \|D_e\Omega_e\|_2
    \nonumber\\
    &\leq
    \lambda
    \|D_e\|_2
    \|\Omega_e\|_2
    \nonumber\\
    &\leq
    \lambda
    \sqrt{H(H-1)}.
    \label{eq:appendix-offdiag-residual-bound}
\end{align}

Thus, for fixed \(H\), \(\lambda\) scales a uniform worst-case bound on the
additional edge transport. This is only a perturbation bound on the
single-edge operator; it does not imply that the complete neural layer is
contractive or provide a stability guarantee for the full network.


\subsection{Relation between the diagonal and residual families}
\label{app:nested-operator-families}

The preceding results make the inclusion between standard attention and
\textsc{TopA} explicit. At a fixed network state, standard attention uses edge
operators of the form
\[
    D_e
    =
    \operatorname{Diag}
    \left(
        \alpha_e^{(1)},\ldots,\alpha_e^{(H)}
    \right),
\]
whereas \textsc{TopA} uses
\[
    T_e
    =
    D_e
    \left(
        I_H+\lambda\Omega_e
    \right),
    \qquad
    \operatorname{diag}(\Omega_e)=0.
\]
The latter retains exactly the same diagonal entries and introduces only
off-diagonal source-to-receiver head routes. Setting
\(\Omega_e=0\), or equivalently taking \(\lambda=0\), returns the diagonal
attention operator.

This inclusion is defined in the native architectural head basis. It is the
specific structural relaxation studied in this work, rather than a claim
that \textsc{TopA} spans the entire space of arbitrary
\(H\times H\) edge operators.
