# Supplementary material for: Let the Heads Talk: Beyond Diagonal Graph Attention
Source: arXiv:2610.01494 source file (2026-10-01)
Supplement: Supplementary file 4 [file appendix_c.tex]

\section{Cellular-Sheaf Realization of \textsc{TopA}}
\label{app:offdiag-sheaf}

This appendix gives the full restriction-induced realization of the
\textsc{TopA} operator introduced in
Section~\ref{sec:offdiag-sheaf-realization}. The construction is
architecture-aligned: its two edge-stalk components correspond directly to
the standard attention path and the residual cross-head routing path.

Throughout this section, fix a layer and network state so that the attention
operators \(D_e\) and routing matrices \(\Omega_e\) are instantiated for all
directed edges. As in the main text,
\begin{equation}
    T_e
    =
    D_e
    \left(
        I_H+\lambda\Omega_e
    \right)
    =
    D_e+\lambda D_e\Omega_e,
    \qquad
    \operatorname{diag}(\Omega_e)=0,
    \label{eq:appendix-offdiag-operator}
\end{equation}
with \(D_e\in\R^{H\times H}\) diagonal and non-negative.


\subsection{Direct-sum edge-stalk construction}
\label{app:offdiag-direct-sum}

For each directed edge \(e=(j\to i)\), assign
\begin{equation}
    \mathcal{F}(j)
    =
    \mathcal{F}(i)
    =
    \R^H
\end{equation}
to the sender and receiver vertices, and choose the edge stalk
\begin{equation}
    \mathcal{F}(e)
    =
    \R^H_{\mathrm{att}}
    \oplus
    \R^H_{\mathrm{route}}
    \cong
    \R^{2H}.
    \label{eq:appendix-offdiag-edge-stalk}
\end{equation}
The first summand will represent the standard attention path, while the
second represents the residual routing path.

Since the normalized attention coefficients are non-negative, the principal
square root
\begin{equation}
    D_e^{1/2}
    =
    \operatorname{Diag}
    \left(
        \sqrt{\alpha_e^{(1)}},
        \ldots,
        \sqrt{\alpha_e^{(H)}}
    \right)
    \label{eq:appendix-offdiag-attention-sqrt}
\end{equation}
is well defined.

Define the sender and receiver restriction maps
\begin{equation}
    S_e:
    \mathcal{F}(j)
    \longrightarrow
    \mathcal{F}(e),
    \qquad
    R_e:
    \mathcal{F}(i)
    \longrightarrow
    \mathcal{F}(e)
\end{equation}
by
\begin{equation}
    S_e
    =
    \begin{bmatrix}
        D_e^{1/2}\\[1mm]
        \sqrt{\lambda}\,\Omega_e
    \end{bmatrix},
    \qquad
    R_e
    =
    \begin{bmatrix}
        D_e^{1/2}\\[1mm]
        \sqrt{\lambda}\,D_e
    \end{bmatrix}.
    \label{eq:appendix-offdiag-restrictions}
\end{equation}
Both maps have shape \(2H\times H\), as required for maps from an
\(H\)-dimensional vertex stalk into the \(2H\)-dimensional edge stalk.


\subsection{Exact realization of the edge operator}
\label{app:proof-offdiag-sheaf}

We now prove
Proposition~\ref{prop:offdiag-sheaf-realization}.

\begin{proof}[Proof of Proposition~\ref{prop:offdiag-sheaf-realization}]
Using the block structure in
Equation~\eqref{eq:appendix-offdiag-restrictions},
\begin{align}
    R_e^\top S_e
    &=
    \begin{bmatrix}
        \left(D_e^{1/2}\right)^\top
        &
        \sqrt{\lambda}\,D_e^\top
    \end{bmatrix}
    \begin{bmatrix}
        D_e^{1/2}\\[1mm]
        \sqrt{\lambda}\,\Omega_e
    \end{bmatrix}
    \nonumber\\
    &=
    \left(D_e^{1/2}\right)^\top
    D_e^{1/2}
    +
    \lambda D_e^\top\Omega_e.
    \label{eq:appendix-offdiag-factorization-step}
\end{align}
Because \(D_e\) is diagonal and non-negative,
\(D_e^{1/2}\) is symmetric and
\[
    \left(D_e^{1/2}\right)^\top
    D_e^{1/2}
    =
    D_e.
\]
Moreover, \(D_e^\top=D_e\). Hence
\begin{align}
    R_e^\top S_e
    &=
    D_e+\lambda D_e\Omega_e
    \nonumber\\
    &=
    D_e
    \left(
        I_H+\lambda\Omega_e
    \right)
    \nonumber\\
    &=
    T_e.
    \label{eq:appendix-offdiag-factorization}
\end{align}

Therefore the source-to-target message induced by the restriction maps is
\begin{equation}
    R_e^\top S_eV_{s(e)}
    =
    T_eV_{s(e)},
\end{equation}
which is exactly the \textsc{TopA} edge message.

Collecting the sender and receiver restrictions into the incidence operators
\(B_s\) and \(B_t\) defined in
Appendix~\ref{app:global-incidence}, we obtain
\begin{align}
    \left(
        B_t^\ast B_sV
    \right)_i
    &=
    \sum_{e:t(e)=i}
    R_e^\top S_eV_{s(e)}
    \nonumber\\
    &=
    \sum_{e:t(e)=i}
    T_eV_{s(e)}
    \nonumber\\
    &=
    M_i^{\offdiag}.
    \label{eq:appendix-offdiag-global-transport}
\end{align}
Thus the complete \textsc{TopA} aggregation is exactly realized by the directed
cross-incidence transport \(B_t^\ast B_s\).
\end{proof}


\subsection{Interpretation of the two edge-stalk components}
\label{app:offdiag-path-decomposition}

The direct-sum construction makes the two computational paths of
Equation~\eqref{eq:appendix-offdiag-operator} explicit. For a sender value
\(V_{s(e)}\), the sender restriction produces
\begin{equation}
    S_eV_{s(e)}
    =
    \begin{bmatrix}
        D_e^{1/2}V_{s(e)}\\[1mm]
        \sqrt{\lambda}\,\Omega_eV_{s(e)}
    \end{bmatrix}.
    \label{eq:appendix-offdiag-sender-lift}
\end{equation}
The upper component carries the standard attention contribution, while the
lower component carries the routed cross-head contribution.

Applying the adjoint receiver restriction gives
\begin{align}
    R_e^\top S_eV_{s(e)}
    &=
    \left(D_e^{1/2}\right)^\top
    D_e^{1/2}V_{s(e)}
    +
    \lambda
    D_e^\top\Omega_eV_{s(e)}
    \nonumber\\
    &=
    D_eV_{s(e)}
    +
    \lambda D_e\Omega_eV_{s(e)}.
    \label{eq:appendix-offdiag-two-path-message}
\end{align}
The first term is exactly the vanilla attention message,
\begin{equation}
    m_e^{\mathrm{att}}
    =
    D_eV_{s(e)},
\end{equation}
while the second is the residual cross-head contribution,
\begin{equation}
    m_e^{\mathrm{route}}
    =
    \lambda D_e\Omega_eV_{s(e)}.
\end{equation}
Their sum is the implemented \textsc{TopA} message.

This decomposition is the reason for using
\(\R^H_{\mathrm{att}}\oplus\R^H_{\mathrm{route}}\): the edge stalk records
the standard and residual pathways separately before they are combined at
the receiver.


\subsection{Action on the full value representation}
\label{app:offdiag-full-value-space}

The restriction maps above act on the \(H\)-dimensional head factor. The
\(C\) coordinates within each head remain parallel signals, as in the main
construction.

On the full value space
\[
    \R^H\otimes\R^C,
\]
the induced transport is therefore
\begin{equation}
    T_e\otimes I_C
    =
    \left[
        D_e
        \left(
            I_H+\lambda\Omega_e
        \right)
    \right]
    \otimes I_C.
    \label{eq:appendix-offdiag-full-space}
\end{equation}
Equivalently, the restriction maps can be lifted as
\begin{equation}
    \widetilde{S}_e
    =
    S_e\otimes I_C,
    \qquad
    \widetilde{R}_e
    =
    R_e\otimes I_C,
\end{equation}
which gives
\begin{align}
    \widetilde{R}_e^\top
    \widetilde{S}_e
    &=
    (R_e^\top S_e)\otimes I_C
    \nonumber\\
    &=
    T_e\otimes I_C.
    \label{eq:appendix-offdiag-kron-factorization}
\end{align}
Thus the cellular-sheaf realization preserves the same separation between
the head and within-head axes used throughout the architecture.


\subsection{The factorization is induced, not learned}
\label{app:offdiag-induced-not-learned}

The restriction maps in
Equation~\eqref{eq:appendix-offdiag-restrictions} are not independent
parameters of the neural network. The implementation learns the routing
matrix through
\[
    \Omega_e
    =
    \operatorname{off}
    \left(
        \tanh g_\theta(\xi_e)
    \right),
\]
while \(D_e\) is produced by the underlying attention mechanism. Once
\(D_e\) and \(\Omega_e\) have been instantiated, the restriction maps
\(R_e\) and \(S_e\) are determined algebraically by
Equation~\eqref{eq:appendix-offdiag-restrictions}.

The cellular-sheaf construction should therefore be understood as an exact
realization of the operator implemented by \textsc{TopA}, rather than as a
separate parameterization used during optimization. No edge stalk or
restriction map needs to be materialized in the forward implementation.


\subsection{Non-uniqueness of the realization}
\label{app:offdiag-factorization-nonunique}

The factorization
\[
    T_e
    =
    R_e^\top S_e
\]
is not unique. In particular, whenever the vertex and edge spaces are all
identified with \(\R^H\), the trivial choice
\begin{equation}
    R_e
    =
    I_H,
    \qquad
    S_e
    =
    T_e
    \label{eq:appendix-offdiag-trivial-factorization}
\end{equation}
also satisfies
\[
    R_e^\top S_e
    =
    T_e.
\]
Many other factorizations are possible, including ones obtained by changing
the intermediate edge coordinates.

The \(2H\)-dimensional edge stalk in
Equation~\eqref{eq:appendix-offdiag-edge-stalk} is therefore not claimed to
be minimal, canonical, or required for the existence of a factorization.
It is chosen because it reflects the architecture:
\[
    T_e
    =
    \underbrace{D_e}_{\text{attention}}
    +
    \underbrace{\lambda D_e\Omega_e}_{\text{routing}}.
\]
The direct sum assigns one edge-space component to each of these two
computational paths and hence provides an interpretable,
architecture-aligned realization.


\subsection{Directionality of the realization}
\label{app:offdiag-sheaf-directionality}

The construction is applied separately to each directed computational edge.
If both
\[
    e_{j\to i}:j\to i
    \qquad\text{and}\qquad
    e_{i\to j}:i\to j
\]
are present, they are represented by distinct edge cells and may instantiate
different attention and routing matrices:
\[
    D_{i\leftarrow j}
    \neq
    D_{j\leftarrow i},
    \qquad
    \Omega_{i\leftarrow j}
    \neq
    \Omega_{j\leftarrow i}^{\top}.
\]
Their corresponding restriction maps are therefore also independent.

For the \(j\to i\) direction,
\begin{equation}
    T_{i\leftarrow j}
    =
    R_{j\to i}^{\top}
    S_{j\to i},
\end{equation}
while the reverse direction uses
\begin{equation}
    T_{j\leftarrow i}
    =
    R_{i\to j}^{\top}
    S_{i\to j}.
\end{equation}
No reciprocity relation between these operators is imposed. As discussed in
Appendix~\ref{app:directed-sheaf-reciprocity}, this independence follows
from representing opposite computational directions by distinct edge cells,
rather than merely orienting a single shared undirected edge.


\subsection{State dependence}
\label{app:offdiag-sheaf-state-dependence}

Both components of the realization may depend on the current network state.
At layer \(\ell\),
\[
    D_e^{(\ell)}
    =
    D_e^{(\ell)}
    \left(
        X^{(\ell)}
    \right),
    \qquad
    \Omega_e^{(\ell)}
    =
    \Omega_e^{(\ell)}
    \left(
        X^{(\ell)}
    \right).
\]
The induced restriction maps are therefore
\begin{equation}
    R_e^{(\ell)}
    =
    \begin{bmatrix}
        \left(D_e^{(\ell)}\right)^{1/2}\\[1mm]
        \sqrt{\lambda}\,D_e^{(\ell)}
    \end{bmatrix},
    \qquad
    S_e^{(\ell)}
    =
    \begin{bmatrix}
        \left(D_e^{(\ell)}\right)^{1/2}\\[1mm]
        \sqrt{\lambda}\,\Omega_e^{(\ell)}
    \end{bmatrix}.
    \label{eq:appendix-offdiag-dynamic-restrictions}
\end{equation}
For each fixed \(X^{(\ell)}\), these maps define the corresponding
restriction-induced cellular-sheaf realization. As the hidden state changes,
a new collection of edge operators and hence a new realization is
instantiated.

This is consistent with the dynamic graph-copresheaf interpretation of
Appendix~\ref{app:dynamic-copresheaf}: the operator applied directly during
message passing is the state-dependent map \(T_e^{(\ell)}\), while the
cellular-sheaf representation provides an exact factorization of that
instantiated operator.


\subsection{Vanilla attention as the zero-routing case}
\label{app:offdiag-sheaf-vanilla-limit}

The cellular-sheaf realization also makes the reduction to standard
attention explicit. If
\[
    \Omega_e=0,
\]
then
\[
    T_e=D_e.
\]
The sender restriction becomes
\[
    S_e
    =
    \begin{bmatrix}
        D_e^{1/2}\\
        0
    \end{bmatrix},
\]
while the receiver restriction remains
\[
    R_e
    =
    \begin{bmatrix}
        D_e^{1/2}\\
        \sqrt{\lambda}\,D_e
    \end{bmatrix}.
\]
The second edge-stalk component contributes nothing to
\(R_e^\top S_e\), leaving
\[
    R_e^\top S_e
    =
    D_e.
\]

Equivalently, when \(\lambda=0\), both restriction maps reduce to
\[
    R_e
    =
    S_e
    =
    \begin{bmatrix}
        D_e^{1/2}\\
        0
    \end{bmatrix},
\]
again yielding the standard attention operator. Thus the restriction-induced
realization respects the same exact vanilla limit as the \textsc{TopA}
architecture itself.
