# Supplementary material for: Let the Heads Talk: Beyond Diagonal Graph Attention
Source: arXiv:2610.01494 source file (2026-10-01)
Supplement: Supplementary file 5 [file appendix_c_protocols.tex]

\section{Experimental Protocols}
\label{app:protocols}

\begin{table}[h]
\centering
\small
\caption{Feature-partition training and model-selection protocol.}
\begin{tabular}{ll}
\toprule
Item & Setting\\
\midrule
Splits & ten fixed 50/25/25 node splits\\
Search & \(H\in\{2,4,8\}\), \(C\in\{16,32,64\}\), layers \(2\)--\(5\)\\
Trials & 36 grid points per model/regime, no pruning\\
Selection & best split-0 validation accuracy\\
Final score & ten-split test accuracy at best-validation checkpoint\\
Partition & head \(h\) constructs projections from feature subset \(h\)\\
Inter-layer paths & head partition preserved in projections, residuals, and skips\\
Post-aggregation readout & dense decoder in both conditions\\
Optimization & dataset/model preset; early stopping on validation loss\\
\bottomrule
\end{tabular}
\end{table}

The architecture grid is exhaustive and is run separately for every dataset, backbone, model variant, and feature condition. The selected split-0 configuration is then evaluated on all ten supplied data splits. Output normalization is enabled throughout.

\todoresult{Insert the final per-dataset learning rates, weight decays, dropout rates, epoch limits, and early-stopping patience from the experiment configurations.}

\begin{table}[h]
\centering
\small
\caption{CLRS training protocol. Each task is trained separately.}
\begin{tabular}{ll@{\qquad}ll}
\toprule
Field & Value & Field & Value\\
\midrule
package & CLRS 2.0.3, patched & updates & 10,000\\
hidden/heads & 128 / 4 & head width & 32\\
batch size & 32 & learning rate & \(10^{-3}\)\\
MP steps & 1 & dropout/weight decay & 0 / 0\\
seeds & 42--51 & evaluation & every 500 steps\\
checkpoint & best validation & train examples & 320,000\\
\bottomrule
\end{tabular}
\end{table}

The canonical CLRS split uses length 16 for training and validation and length 64 for test. Although 2,048 validation and test samples are requested, canonical availability caps evaluation at 32 trajectories for 22 completed tasks, 1,024 for Kadane, and 2,048 for binary search, minimum, quickselect, KMP, naive string matching, and segments intersect. Seed-level intervals therefore summarize training variation under the fixed benchmark test sets.
