# Supplementary material for: Let the Heads Talk: Beyond Diagonal Graph Attention
Source: arXiv:2610.01494 source file (2026-10-01)
Supplement: Supplementary file 6 [file appendix_d.tex]

\section{Post-Aggregation Equivalence and Implementation Checks}
\label{app:postaggregation-implementation}

This appendix provides the full proof of the post-aggregation equivalence
result from Section~\ref{sec:offdiag-postmix} and records the implementation
checks used to ensure that \textsc{TopA} is an exact residual extension of its
attention backbone. We first lift the head-space operators to the complete
value representation, then characterize when edge-conditioned
pre-aggregation transport can be represented by a single linear map after
aggregation. We finally detail the zero-initialization, gradient behavior,
parameterization, and computational checks used in the implementation.


\subsection{Lifting head-space transport to the full value space}
\label{app:postmix-lifting}

Let
\[
    V
    =
    \begin{bmatrix}
        (V^{(1)})^\top\\
        \vdots\\
        (V^{(H)})^\top
    \end{bmatrix}
    \in\R^{H\times C}.
\]
We define the head-major vectorization
\begin{equation}
    \operatorname{hvec}(V)
    =
    \begin{bmatrix}
        (V^{(1)})^\top &
        \cdots &
        (V^{(H)})^\top
    \end{bmatrix}^{\top}
    \in\R^{HC}.
    \label{eq:appendix-head-vectorization}
\end{equation}
For any \(Q\in\R^{H\times H}\),
\begin{equation}
    \operatorname{hvec}(QV)
    =
    (Q\otimes I_C)
    \operatorname{hvec}(V).
    \label{eq:appendix-head-kron-identity}
\end{equation}

To see this, the \(r\)-th row of \(QV\) is
\[
    (QV)^{(r)}
    =
    \sum_{s=1}^{H}
    Q^{rs}V^{(s)}.
\]
Stacking these rows produces exactly the block action of
\(Q\otimes I_C\) on
\(\operatorname{hvec}(V)\).

Thus the attention and \textsc{TopA} operators acting on the complete value
space are
\begin{equation}
    \overline{D}_{i\leftarrow j}
    =
    D_{i\leftarrow j}\otimes I_C,
    \qquad
    \overline{T}_{i\leftarrow j}
    =
    T_{i\leftarrow j}\otimes I_C.
    \label{eq:appendix-lifted-operators}
\end{equation}
This lifting makes explicit that both operators act on the head factor and
leave the \(C\) within-head coordinates unchanged.


\subsection{Proof of shared post-aggregation equivalence}
\label{app:proof-postmix}

We now prove
Theorem~\ref{thm:postmix-non-equivalence}.

\begin{proof}[Proof of Theorem~\ref{thm:postmix-non-equivalence}]
Fix a receiver \(i\), and suppose there exists
\(A\in\R^{HC\times HC}\) such that
\begin{equation}
    \sum_{j\in\mathcal{N}(i)}
    \overline{T}_{i\leftarrow j}v_j
    =
    A
    \sum_{j\in\mathcal{N}(i)}
    \overline{D}_{i\leftarrow j}v_j
    \label{eq:appendix-postmix-assumption}
\end{equation}
for every collection
\(\{v_j\in\R^{HC}\}_{j\in\mathcal{N}(i)}\).

Choose an arbitrary sender
\(k\in\mathcal{N}(i)\), set
\[
    v_j=0
    \qquad
    \text{for all }j\neq k,
\]
and leave \(v_k\) arbitrary. Equation~\eqref{eq:appendix-postmix-assumption}
then becomes
\[
    \overline{T}_{i\leftarrow k}v_k
    =
    A\,
    \overline{D}_{i\leftarrow k}v_k.
\]
Because this equality holds for every
\(v_k\in\R^{HC}\),
\[
    \overline{T}_{i\leftarrow k}
    =
    A\,
    \overline{D}_{i\leftarrow k}.
\]
Since \(k\) was arbitrary,
\begin{equation}
    \overline{T}_{i\leftarrow j}
    =
    A\,
    \overline{D}_{i\leftarrow j}
    \qquad
    \text{for every }j\in\mathcal{N}(i).
    \label{eq:appendix-common-factor-necessity}
\end{equation}

Conversely, suppose
Equation~\eqref{eq:appendix-common-factor-necessity} holds for every incoming
edge. Then
\begin{align}
    \sum_{j\in\mathcal{N}(i)}
    \overline{T}_{i\leftarrow j}v_j
    &=
    \sum_{j\in\mathcal{N}(i)}
    A\,
    \overline{D}_{i\leftarrow j}v_j
    \nonumber\\
    &=
    A
    \sum_{j\in\mathcal{N}(i)}
    \overline{D}_{i\leftarrow j}v_j,
\end{align}
which proves the required post-aggregation representation.
\end{proof}

The theorem therefore gives an exact necessary and sufficient condition:
all incoming routed operators must admit the \emph{same} left factor relative
to their corresponding attention operators.


\subsection{Specialization to \textsc{TopA}}
\label{app:postmix-offdiag}

For \textsc{TopA},
\begin{equation}
    T_{i\leftarrow j}
    =
    D_{i\leftarrow j}
    \left(
        I_H+\lambda\Omega_{i\leftarrow j}
    \right),
\end{equation}
and hence
\begin{equation}
    \overline{T}_{i\leftarrow j}
    =
    \left[
        D_{i\leftarrow j}
        \left(
            I_H+\lambda\Omega_{i\leftarrow j}
        \right)
    \right]
    \otimes I_C.
    \label{eq:appendix-lifted-offdiag}
\end{equation}

For a present edge with finite softmax logits,
\[
    \alpha_{i\leftarrow j}^{(h)}>0
    \qquad
    \text{for every head }h.
\]
The diagonal matrix \(D_{i\leftarrow j}\) is therefore invertible, with
\[
    D_{i\leftarrow j}^{-1}
    =
    \operatorname{Diag}
    \left(
        \frac{1}{\alpha_{i\leftarrow j}^{(1)}},
        \ldots,
        \frac{1}{\alpha_{i\leftarrow j}^{(H)}}
    \right).
\]
Consequently,
\[
    \overline{D}_{i\leftarrow j}^{-1}
    =
    D_{i\leftarrow j}^{-1}\otimes I_C.
\]

The common-factor condition of
Theorem~\ref{thm:postmix-non-equivalence} then requires
\begin{align}
    A
    &=
    \overline{T}_{i\leftarrow j}
    \overline{D}_{i\leftarrow j}^{-1}
    \nonumber\\
    &=
    \left[
        D_{i\leftarrow j}
        \left(
            I_H+\lambda\Omega_{i\leftarrow j}
        \right)
        D_{i\leftarrow j}^{-1}
    \right]
    \otimes I_C
    \label{eq:appendix-offdiag-left-factor}
\end{align}
for every sender \(j\in\mathcal{N}(i)\).

Thus a single post-aggregation map can reproduce the routed
pre-aggregation representation if and only if the matrices
\begin{equation}
    D_{i\leftarrow j}
    \left(
        I_H+\lambda\Omega_{i\leftarrow j}
    \right)
    D_{i\leftarrow j}^{-1}
    \label{eq:appendix-induced-postmix-factors}
\end{equation}
are identical across all incoming edges.

Edge-conditioned routing imposes no such constraint: both
\(D_{i\leftarrow j}\) and
\(\Omega_{i\leftarrow j}\) may vary with the sender. The routed operator
therefore cannot, in general, be absorbed into one shared linear
transformation after aggregation.

The invertibility argument is only a convenient specialization of the
general theorem. If hard masking, sparse normalization, or another attention
mechanism produces zero diagonal entries, one simply returns to the original
condition
\[
    \overline{T}_{i\leftarrow j}
    =
    A\overline{D}_{i\leftarrow j},
\]
which does not require
\(\overline{D}_{i\leftarrow j}\) to be invertible.


\subsection{Two-edge counterexample}
\label{app:postmix-counterexample}

A minimal example illustrates the failure of shared post-aggregation mixing.
Consider a receiver \(i\) with two incoming edges \(j_1\to i\) and
\(j_2\to i\), and suppose
\begin{equation}
    D_{i\leftarrow j_1}
    =
    D_{i\leftarrow j_2}
    =
    \frac{1}{2}I_H.
    \label{eq:appendix-counterexample-attention}
\end{equation}
This is consistent with each head assigning equal normalized attention to the
two incoming edges.

Let the first edge use no cross-head routing,
\[
    \Omega_{i\leftarrow j_1}=0,
\]
while the second uses a non-zero off-diagonal matrix
\[
    \Omega_{i\leftarrow j_2}
    =
    \Omega,
    \qquad
    \Omega\neq0.
\]
For the first edge,
\[
    T_{i\leftarrow j_1}
    =
    \frac{1}{2}I_H,
\]
so the common-factor condition requires
\begin{equation}
    A
    =
    I_H\otimes I_C.
    \label{eq:appendix-counterexample-first-A}
\end{equation}
For the second edge,
\[
    T_{i\leftarrow j_2}
    =
    \frac{1}{2}
    \left(
        I_H+\lambda\Omega
    \right),
\]
and therefore
\begin{equation}
    A
    =
    \left(
        I_H+\lambda\Omega
    \right)
    \otimes I_C.
    \label{eq:appendix-counterexample-second-A}
\end{equation}
Whenever
\[
    \lambda\Omega\neq0,
\]
Equations~\eqref{eq:appendix-counterexample-first-A} and
\eqref{eq:appendix-counterexample-second-A} are incompatible. No single
post-aggregation linear map can therefore reproduce both edge-specific
transformations.


\subsection{Scope of the equivalence result}
\label{app:postmix-scope}

Theorem~\ref{thm:postmix-non-equivalence} is an operator-level statement
about a fixed receiver in a single instantiated attention layer. It compares
two computations:

\begin{enumerate}
    \item applying a potentially different operator
    \(\overline{T}_{i\leftarrow j}\) to each sender before aggregation; and
    \item aggregating with the standard attention operators
    \(\overline{D}_{i\leftarrow j}\) and then applying one linear map \(A\).
\end{enumerate}

The theorem is deliberately generous to the post-aggregation alternative:
\(A\) is allowed to be an arbitrary \(HC\times HC\) matrix and may be chosen
separately for the fixed receiver \(i\). A conventional output projection
\(W_O\) is typically shared across receivers, so it satisfies an even
stronger sharing constraint.

The result should nevertheless not be interpreted as a universal
function-class separation between complete deep networks. Subsequent layers,
nonlinearities, additional message-passing steps, or alternative
architectures may approximate or realize related functions through different
computational paths. The theorem establishes the narrower fact needed here:
for fixed instantiated edge maps, edge-specific pre-aggregation transport
cannot in general be rewritten as one shared linear transformation of the
standard aggregated representation.

Likewise, if a non-injective downstream readout discards distinctions between
two pre-readout representations, the final outputs may coincide for
particular inputs. The theorem concerns exact reconstruction of the routed
pre-readout representation for all sender values.


\subsection{Exact vanilla reference point}
\label{app:implementation-vanilla-reference}

The implementation uses the dense routing projection
\begin{equation}
    G_e
    =
    \operatorname{reshape}_{H\times H}
    \left(
        W_\Omega\xi_e+b_\Omega
    \right),
    \qquad
    \Omega_e
    =
    \operatorname{off}
    \left(
        \tanh G_e
    \right).
    \label{eq:appendix-routing-implementation}
\end{equation}

There are two useful vanilla reference configurations.

\paragraph{Explicit vanilla baseline.}
The routing branch is absent and the edge operator is
\begin{equation}
    T_e^{\mathrm{base}}
    =
    D_e.
    \label{eq:appendix-explicit-vanilla}
\end{equation}
No routing parameters are present.

\paragraph{Zero-initialized \textsc{TopA}.}
In the active model, the routing branch is retained but initialized with
\begin{equation}
    W_\Omega=0,
    \qquad
    b_\Omega=0.
    \label{eq:appendix-zero-init}
\end{equation}
For every edge descriptor \(\xi_e\),
\begin{align}
    G_e
    &=
    0,
    \nonumber\\
    \Omega_e
    &=
    \operatorname{off}(\tanh 0)
    =
    0,
    \nonumber\\
    T_e
    &=
    D_e.
    \label{eq:appendix-zero-init-chain}
\end{align}
Thus, for identical shared-backbone parameters,
\begin{equation}
    M_i^{\offdiag}
    =
    M_i^{\att}
    \qquad
    \text{at initialization}.
    \label{eq:appendix-initial-forward-equivalence}
\end{equation}
All subsequent backbone operations therefore also receive identical inputs,
so the two networks implement exactly the same function at the initial
parameter state.

This equivalence is stronger than simply choosing a small initial routing
matrix: the initial residual contribution is identically zero on every edge.


\subsection{First-order learning from the vanilla solution}
\label{app:implementation-gradient}

Zero initialization does not create a first-order barrier to learning the
off-diagonal routes. Let
\(E^{rs}\in\R^{H\times H}\) denote the matrix with a single unit entry at
\((r,s)\). At \(G_e=0\), the derivative of the elementwise \(\tanh\) is one.
After the diagonal mask,
\begin{equation}
    \left.
    \frac{\partial \Omega_e}
         {\partial G_e^{rs}}
    \right|_{G_e=0}
    =
    \begin{cases}
        E^{rs}, & r\neq s,\\
        0,      & r=s.
    \end{cases}
    \label{eq:appendix-omega-local-derivative}
\end{equation}
For \(r\neq s\),
\begin{align}
    \left.
    \frac{\partial T_e}
         {\partial G_e^{rs}}
    \right|_{G_e=0}
    &=
    \lambda D_eE^{rs},
    \label{eq:appendix-transport-local-derivative}
\end{align}
and hence
\begin{equation}
    \left.
    \frac{\partial(T_eV_j)}
         {\partial G_e^{rs}}
    \right|_{G_e=0}
    =
    \lambda
    D_eE^{rs}V_j.
    \label{eq:appendix-message-local-derivative}
\end{equation}
In component form, this derivative contributes to receiver row \(r\) as
\begin{equation}
    \lambda
    \alpha_e^{(r)}
    V_j^{(s)}.
    \label{eq:appendix-route-first-order-signal}
\end{equation}
Thus the parameterization permits a non-zero first-order learning signal for
every off-diagonal route whenever the corresponding value and downstream
gradient are non-zero.

The diagonal generator outputs receive no gradient because they are removed
by \(\operatorname{off}(\cdot)\).

There is also no additional first-order gradient into the shared backbone
through the routing descriptor at initialization. Since
\[
    G_e=W_\Omega\xi_e+b_\Omega
\]
and \(W_\Omega=0\),
\begin{equation}
    \left.
    \frac{\partial G_e}{\partial \xi_e}
    \right|_{\mathrm{init}}
    =
    W_\Omega
    =
    0.
\end{equation}
Hence the new routing path initially contributes no gradient to the
representations used to construct \(\xi_e\). The shared backbone therefore
starts from the same forward computation and the same routing-induced
gradient contribution as vanilla attention, while the new parameters
\(W_\Omega\) and \(b_\Omega\) are free to move away from zero.

For \(\lambda=0\), both the routed contribution and its parameter gradients
vanish. The principal experiments use a non-zero routing scale.


\subsection{Receiver-gated implementation order}
\label{app:implementation-order}

A critical implementation detail is the ordering
\begin{equation}
    T_e
    =
    D_e
    \left(
        I_H+\lambda\Omega_e
    \right),
    \label{eq:appendix-receiver-gated-order}
\end{equation}
rather than
\[
    (I_H+\lambda\Omega_e)D_e.
\]
The implemented message can equivalently be evaluated as
\begin{equation}
    m_e
    =
    D_e
    \left(
        V_j+\lambda\Omega_eV_j
    \right).
    \label{eq:appendix-message-computation-order}
\end{equation}
For receiver head \(r\),
\begin{equation}
    m_e^{(r)}
    =
    \alpha_e^{(r)}
    \left[
        V_j^{(r)}
        +
        \lambda
        \sum_{s\neq r}
        \Omega_e^{rs}V_j^{(s)}
    \right].
    \label{eq:appendix-component-order-check}
\end{equation}
The attention coefficient of receiver head \(r\) therefore gates every
contribution entering that head. This equation is also used as a componentwise
check of the matrix implementation.


\subsection{Implementation invariants and parity checks}
\label{app:implementation-parity}

The implementation is checked against several invariants implied by the
theory.

\paragraph{Zero diagonal.}
After the routing projection,
\begin{equation}
    \operatorname{diag}(\Omega_e)=0
\end{equation}
for every edge. Consequently,
\[
    \operatorname{diag}(T_e)
    =
    \operatorname{diag}(D_e).
\]

\paragraph{Head-space action only.}
For \(V_j\in\R^{H\times C}\), the routing multiplication is performed along
the \(H\)-dimensional head axis:
\[
    \Omega_eV_j
    \in
    \R^{H\times C}.
\]
No edge-dependent \(C\times C\) channel transformation is introduced. On
the vectorized value space, the implemented operator is therefore
\(T_e\otimes I_C\).

\paragraph{Disabled-routing parity.}
With the routing branch explicitly disabled, the model uses exactly
\[
    T_e=D_e
\]
and the same value projections, attention coefficients, aggregation,
residual paths, nonlinearities, and normalization as the corresponding
backbone.

\paragraph{Zero-initialization parity.}
With the routing branch active but
\(W_\Omega=b_\Omega=0\), we verify that the generated routing matrices vanish
and that the edge messages, aggregated representations, and final model
outputs agree with the corresponding vanilla computation for the same shared
parameters.

These checks are applied to both backbone instantiations. They verify the
implementation of the operator itself rather than relying only on equal
training configurations.

The active \textsc{TopA} model contains additional routing parameters, so the
comparison is functionally matched at initialization but is not
parameter-count matched unless an additional capacity-matched control is
introduced.


\subsection{Routing parameter count}
\label{app:implementation-parameters}

For a descriptor
\[
    \xi_e\in\R^p,
\]
the dense generator in
Equation~\eqref{eq:appendix-routing-implementation} uses
\[
    W_\Omega
    \in
    \R^{H^2\times p},
    \qquad
    b_\Omega
    \in
    \R^{H^2}.
\]
The allocated number of routing parameters per layer is therefore
\begin{equation}
    N_{\mathrm{route}}
    =
    pH^2+H^2
    =
    H^2(p+1).
    \label{eq:appendix-route-parameter-count}
\end{equation}

Because the diagonal of the generated matrix is subsequently masked, only
\(H(H-1)\) output coordinates affect the model. The number of active
off-diagonal generator parameters is therefore
\begin{equation}
    N_{\mathrm{route}}^{\mathrm{active}}
    =
    H(H-1)(p+1),
    \label{eq:appendix-active-route-parameters}
\end{equation}
although the implementation retains the dense \(H^2\)-output projection for
simplicity.

For the GATv2 descriptor in
Section~\ref{sec:offdiag-gatv2},
\(\xi_e\) has the same width as the full multi-head edge context. When this
width is \(HC\),
\begin{equation}
    p=HC,
    \qquad
    N_{\mathrm{route}}
    =
    H^3C+H^2.
    \label{eq:appendix-gatv2-route-parameters}
\end{equation}

For the graph Transformer descriptor
\[
    \xi_{i\leftarrow j}
    =
    \operatorname{vec}
    \left(
        Q_i\Vert K_{i\leftarrow j}
    \right),
\]
both \(Q_i\) and \(K_{i\leftarrow j}\) contain \(HC\) coordinates, giving
\begin{equation}
    p=2HC,
    \qquad
    N_{\mathrm{route}}
    =
    2H^3C+H^2.
    \label{eq:appendix-gt-route-parameters}
\end{equation}

For multiple processor layers with independent routing projections, the
total routing parameter count is the sum of
Equation~\eqref{eq:appendix-route-parameter-count} over layers.


\subsection{Detailed computational and memory cost}
\label{app:implementation-complexity}

Generating the dense routing matrix requires a multiplication from
\(\R^p\) to \(\R^{H^2}\), giving
\begin{equation}
    O(pH^2)
\end{equation}
operations per directed edge. The elementwise nonlinearity and diagonal mask
require
\[
    O(H^2).
\]

Applying the cross-head matrix to the sender values,
\[
    \Omega_eV_j,
    \qquad
    \Omega_e\in\R^{H\times H},
    \quad
    V_j\in\R^{H\times C},
\]
costs
\begin{equation}
    O(H^2C)
\end{equation}
operations per edge. The subsequent elementwise multiplication by the
receiver-head attention coefficients contributes \(O(HC)\), which is lower
order than dense head routing when \(H>1\).

Excluding computations already performed by the backbone to construct
\(\xi_e\), the total additional graph-level complexity is therefore
\begin{equation}
    O\!\left(
        |\mathcal{E}|\,pH^2
        +
        |\mathcal{E}|\,H^2C
    \right).
    \label{eq:appendix-total-routing-complexity}
\end{equation}

If every routing matrix is materialized simultaneously, storing
\(\Omega_e\) for all directed edges requires
\begin{equation}
    O(|\mathcal{E}|H^2)
    \label{eq:appendix-routing-memory}
\end{equation}
additional memory. Implementations that generate and consume routing
matrices in chunks can reduce the peak materialization cost without changing
the operator.

The quadratic dependence on \(H\) is a direct consequence of allowing every
source head to route to every receiver head on each edge. The architecture
studied in this work uses this dense form deliberately; sparsity, low-rank
routing, or structured head graphs would define different parameterizations
and are not required for the present construction.


\subsection{Summary of the implementation correspondence}
\label{app:implementation-correspondence}

The implementation can be summarized by the sequence
\begin{equation}
    \xi_e
    \xrightarrow{\;W_\Omega,b_\Omega\;}
    G_e
    \xrightarrow{\;\tanh,\operatorname{off}\;}
    \Omega_e
    \xrightarrow{\;D_e(I_H+\lambda\Omega_e)\;}
    T_e
    \xrightarrow{\;V_{s(e)}\;}
    m_e.
    \label{eq:appendix-routing-pipeline}
\end{equation}
The corresponding structural constraints are
\[
    \operatorname{diag}(\Omega_e)=0,
    \qquad
    \operatorname{diag}(T_e)=\operatorname{diag}(D_e),
\]
and
\[
    W_\Omega=b_\Omega=0
    \quad\Longrightarrow\quad
    T_e=D_e.
\]

Thus the implemented architecture matches the theoretical object analyzed in
Sections~\ref{sec:native} and~\ref{sec:methodology}: a dense,
edge-conditioned transformation of the native head axis applied before
neighborhood aggregation, with standard attention recovered exactly at the
zero-routing solution.
