# Supplementary material for: Let the Heads Talk: Beyond Diagonal Graph Attention
Source: arXiv:2610.01494 source file (2026-10-01)
Supplement: Supplementary file 7 [file appendix_d_feature_splitting.tex]

\section{Full Feature-Partition Diagnostics}
\label{app:fixed-feature-partition}

\begin{table}[ht]
\centering
\small
\caption{Median validation difference (partitioned minus dense, percentage points) across the matched 36-point architecture grid.}
\begin{tabular}{lrrrr}
\toprule
Dataset & GATv2 & OffDiag-GATv2 & GT & OffDiag-GT\\
\midrule
Roman Empire & -13.9 & -2.7 & -7.2 & +0.4\\
Amazon Ratings & -1.9 & +3.4 & +0.0 & +0.6\\
Squirrel Filtered & -0.2 & +2.0 & -0.6 & +1.1\\
Chameleon Filtered & -0.3 & +4.0 & -0.2 & +3.0\\
\bottomrule
\end{tabular}
\end{table}

Across the matched grid, the median partition effect is less negative for the OffDiag variant in all eight dataset--backbone comparisons. This diagnostic complements the selected-configuration interaction in Table~\ref{tab:feature-main}; it is not the primary estimand because grid points differ in capacity and depth.

\todoresult{Add paired split-level confidence intervals, random feature partitions, and the complete selected hyperparameter table.}
