# Supplementary material for: Let the Heads Talk: Beyond Diagonal Graph Attention
Source: arXiv:2610.01494 source file (2026-10-01)
Supplement: Supplementary file 8 [file appendix_e_clrs.tex]

\section{Full CLRS Results}
\label{app:clrs}

\begingroup
\footnotesize
\setlength{\tabcolsep}{1.5pt}
\input{tables/clrs_all_tasks.tex}
\endgroup

\paragraph{Overall uncertainty.}
The primary difference is the mean of 29 task-level paired means. A hierarchical bootstrap (fixed seed 20260721, 10,000 replicates) resamples tasks and then paired seed differences within each selected task, producing \([\ClrsBootLo,\ClrsBootHi]\) percentage points. This interval captures observed task heterogeneity and training variation without treating all 290 task--seed cells as exchangeable independent observations.

\paragraph{Failure accounting.}
All 20 intended \texttt{optimal\_bst} runs fail before producing a score: ten seeds for each processor encounter the same JAX reshape error from a \(512\times1\) tensor to \(1\times1\times1\times32\times32\). We therefore exclude the task symmetrically and report CLRS-29 rather than imputing results.
