# Supplementary material for: Let the Heads Talk: Beyond Diagonal Graph Attention
Source: arXiv:2610.01494 source file (2026-10-01)
Supplement: Supplementary file 9 [file appendix_f_standard_benchmarks.tex]

\section{Supplementary Standard Graph Benchmarks}
\label{app:benchmarks}

\begin{table}[h]
\centering
\small
\caption{Standard-benchmark test accuracy (\%, mean \(\pm\) standard deviation over paired splits), with parameters, runtime, and peak memory reported for each model.}
\label{tab:standard-benchmarks}
\begin{tabular}{lccccc}
\toprule
Dataset & GATv2 & OffDiag-GATv2 & GT & OffDiag-GT & SNN baselines\\
\midrule
\multicolumn{6}{c}{\emph{TODO: insert paired benchmark results}}\\
\bottomrule
\end{tabular}
\end{table}

\todoresult{Populate Table~\ref{tab:standard-benchmarks} from a common paired protocol on homophilous and heterophilous node-classification datasets.}
