# Supplementary material for: Let the Heads Talk: Beyond Diagonal Graph Attention
Source: arXiv:2610.01494 source file (2026-10-01)
Supplement: Supplementary file 10 [file appendix_g_routing_analysis.tex]

\section{Routing-Analysis Details}
\label{app:routing}

\begin{table}[h]
\centering
\small
\caption{Metrics and interventions for the learned-routing analysis.}
\begin{tabular}{lll}
\toprule
Question & Metric/intervention & Aggregation\\
\midrule
Is routing off-diagonal? & \(\rho_{\off}\), signed/absolute route & layer and split\\
Is routing concentrated? & row entropy, top-route mass & edge then layer\\
How many routes matter? & singular spectrum, effective rank & edge then graph\\
Do heads reorganize? & covariance, correlation, linear CKA & aligned heads\\
Is routing necessary? & identity and diagonal-only interventions & paired score drop\\
Is edge specificity necessary? & edge shuffle and layer mean & paired score drop\\
\bottomrule
\end{tabular}
\end{table}

\paragraph{Trace protocol.}
Use the best-validation checkpoint for each of the ten splits and freeze all weights. Sample the same evaluation edges for dense and partitioned conditions. Record projected values, normalized attention, \(O\), routed edge messages, and post-aggregation head states. Compute edge metrics before averaging, retaining signed and absolute summaries. Align heads on a held-out reference split and report sensitivity to the alignment procedure.

For a receiver-head row \(r\), define route probabilities from magnitudes,
\[
p_{rs}=\frac{|O^{rs}|}{\sum_{t\ne r}|O^{rt}|+\epsilon},\qquad s\ne r,
\]
and report normalized entropy together with top-route mass. For singular values \(\sigma_k\), normalize \(q_k=\sigma_k/\sum_\ell\sigma_\ell\) and use \(\exp(-\sum_k q_k\log q_k)\) as effective rank.

\todoresult{Insert the complete routing-statistic table and layer-wise plots.}

\paragraph{Intervention protocol.}
For an intact operator \(P=D+O\), evaluate \(I\), \(D\), a permutation of \(O\) across edges within each graph, and \(D+\bar O\) using the layerwise mean. Do not retrain after intervention. The unit of inference is the data split; report the intact-minus-intervened difference and a paired 95\% interval. Roman Empire is primary, Amazon Ratings secondary, and the two filtered datasets exploratory.

\todoresult{Insert intact-minus-intervened accuracy changes and paired intervals.}

\paragraph{Covariance and CKA.}
At each traced stage, represent head \(h\) by a sample-by-feature matrix \(X_h\) on a common sample axis. Report the \(H\times H\) covariance and correlation matrices, mean absolute off-diagonal correlation, and the effective rank of the head covariance. Linear CKA is computed between centered \(X_h\) matrices after head alignment. All summaries are reported by layer and feature condition.

\todoresult{Insert covariance, correlation, effective-rank, and CKA results for Roman Empire and Amazon Ratings.}
